# Supplementary material for: Detecting induced $p \pm ip$ pairing at the Al-InAs interface with a quantum microwave circuit
Source: arXiv:2107.03695 source file (2022-05-11)
Supplement: Supplementary file 1 [file supplement.pdf]

# Supplementary materials for: Detecting induced $p \pm ip$ pairing at the Al-InAs interface with a quantum microwave circuit


D. Phan,[1] J. Senior,[1] A. Ghazaryan,[1] M. Hatefipour,[2]
W. M. Strickland,[2] J. Shabani,[2] M. Serbyn,[1] and A. P. Higginbotham[1]

[1] *IST Austria, Am Campus 1, 3400 Klosterneuburg, Austria*
[2] *Department of Physics, New York University, New York, NY, 10003, USA*



(Dated: May 11, 2022)


## CONTENTS


I. Analysis overview 1
  A. Summary of equations used for fitting 1
  B. Derivation of expressions for $c_s$ and $c_p$ 2
  C. Analysis steps 3

II. Additional datasets 4
  A. Error estimates 5
  B. Effect of reduced induced gap 5
  C. Fit for $g_y$ 5
  D. Effect of spin-orbit coupling 5
  E. Crystal orientation tunes anisotropy 7
  F. InAs heterostructure causes anisotropy 8
  G. InAs heterostructure causes abrupt increase in dissipation 8
  H. Power dependence of the resonant frequency and quality factor 8
  I. Line cuts of $n_p(B, T)$ 11
  J. Cartesian field-angle plots 11

III. Further experimental information 11
  A. Material Growth 11
  B. Magnetic field alignment 12
  C. Sample Fabrication 12

IV. Theory for superfluid density and dissipation 13
  A. Depairing theory of aluminum superconductivity 13
  B. Superfluid density in p-wave superconductor 15
    1. Model for InAs 15
    2. Bogoliubov Fermi surfaces 15
    3. Electromagnetic response of InAs layer 16
    4. Superfluid density without spin-orbit coupling 18
  C. Dissipation in Al 18

  References 19


## I. ANALYSIS OVERVIEW

### A. Summary of equations used for fitting

In this section we give a self-contained overview of data analysis procedures used in the main text. Based on the circuit model, the geometric and kinetic contributions to the resonant frequency sum in inverse quadrature [1, 2]

$$\frac{1}{f_r^2} = \frac{1}{f_{\mathrm{geo}}^2} + \frac{1}{f_{\mathrm{kin}}^2}, \tag{S1}$$

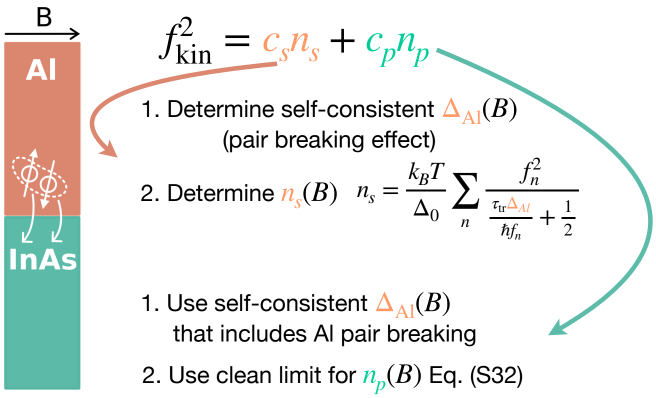


Figure S1: $n_s$ is determined from the self-consistent expression for $\Delta_{\text{Al}}(B)$, and thus includes pair breaking. The induced gap in the InAs is assumed to be equal to $\Delta_{\text{Al}}(B)$. Bogoliubov-Fermi surfaces therefore emerge when $g\mu_B B > \Delta_{\text{Al}}(B)$. $n_p$ is calculated in the clean limit, and therefore does not explicitly include pair-breaking effects of the InAs, *i.e.* $n_p = 1$ for $g\mu_B B < \Delta_{\text{Al}}(B)$ and $T = 0$.

where $f_r$ is the circuit resonant frequency, $f_{\text{geo}}$ is the geometric resonant frequency of the circuit, and $f_{\text{kin}}$ is the kinetic contribution. The kinetic inductance has parallel contributions from the Al and InAs. Equivalently, the total superfluid density is the sum of contributions from the Al and InAs. The kinetic contribution depends on the normalized $s$-wave superfluid density, $n_s$, the normalized $p$-wave superfluid density $n_p$, and constants $c_s$ ($c_p$) as

$$f_{\text{kin}}^2(B,T) = c_s n_s \left( \frac{T_c(B)}{T_{c,0}}, \frac{T}{T_{c,0}} \right) + c_p n_p \left( \frac{T_c(B)}{T_{c,0}}, \frac{g\mu_b B}{\Delta}, \frac{k_b T}{\Delta} \right), \tag{S2}$$

where we explicitly listed dependence of all quantities on temperature, magnetic field and other parameters. Here $\Delta = \Delta\left(\frac{T_c(B)}{T_{c,0}}, \frac{T}{T_{c,0}}\right)$ denotes the self-consistent value of the gap in Al which depends on the magnetic field and temperature and is calculated from Eq. (S16). Thus, pair-breaking effects are included for the Al film, but not for the InAs, as summarized in Fig. S1.

The value of the proximity-induced gap in InAs is assumed to coincide with the Al gap, which is reasonable for a thin quantum well with a disordered superconductor [3]. The dimensionless functions $n_s$ and $n_p$ are listed in Eq. (S17) and Eq. (S32) respectively. Finally, the numerical constants $c_s$ and $c_p$ are listed in Eq. (S9). In practice, their value is determined numerically from fitting procedure, and later the Eq. (S9) is used to translate values of $c_{s,p}$ into physical characteristics of Al and InAs, such as sheet resistance, density, and mobility.

We note that the peculiar dependence of superfluid density $n_s$ in Eq. (S2) on magnetic field that enters via the critical temperature, $T_c(B)$ normalized by the zero-field value, $T_{c,0} \equiv T_c(B = 0)$, comes from the pair-breaking theory of Al. The universal nature of pair-breaking suppression of superconductivity that holds in certain regime of parameters, allows to express all quantities via pair-breaking parameter $\alpha(T_c(B)/T_{c,0})$, see Sec. IV A for a detailed discussion. In contrast, the $n_p$ also depends directly on the value of the magnetic field, see Sec. IV B.

The direction-dependent $g$-factor used in Fig. 4 is defined as [4, 5]: $g((b)) = \frac{1}{|B|}\sqrt{g_x^2 B_x^2 + g_y^2 B_y^2}$, where $B_y = B \sin\theta$, and $g_y$ is the $g$-factor in the $\theta = 90°$ direction.

The theoretical expression for the internal quality factor in Fig. 5(a) is

$$Q_i = \frac{1}{\alpha} \frac{\sigma_2}{\sigma_1}, \tag{S3}$$

where $\alpha$ is the quotient of the kinetic and the total inductance, $\alpha = L_{\text{kin}}/L_{\text{total}}$, and non-dissipative ($\sigma_2$) and dissipative ($\sigma_1$) conductivities normalized by the conductivity of the normal state are given by Eq.'s

### B. Derivation of expressions for $c_s$ and $c_p$

To derive explicit expressions for constants $c_{s,p}$ we start with the thin-film expression for kinetic sheet inductance for each component, $L_\square = \mu_0 \lambda^2/d$ [2], where $\lambda$ is the penetration depth and $d$ is the film thickness. The inductance

per unit length is $\gamma L_\square$ where $\gamma$ is a geometric factor. The value of $\gamma$ is determined by the width of the coplanar waveguide resonator center line denoted as $s$, the gap to the ground plane, $w$, and the thickness of the film, $d$ [2, 6]:

$$\gamma = \frac{(s+2w)^2}{32K(k_0)w(s+w)}\left(\frac{1}{s}\ln\left(\frac{s}{\delta}\frac{w}{s+w}\right)+\frac{1}{s+2w}\ln\left(\frac{s+2w}{\delta}\frac{w}{s+w}\right)\right), \tag{S4}$$

where $\delta = d/(4\pi e^\pi)$ is rescaled thickness of the film, dimensionless parameter $k_0$ is equal to $k_0 = s/(s+2w)$, and $K(k_0)$ is the value of complete elliptic integral of the first kind. In our two-component system there is a sheet inductance from both the Al and the InAs, and for both we take a nominal thickness of $d = 15$ nm. The results are, however, not very sensitive to this assumption; taking for InAs the quantum-well width 7 nm changes $\gamma$ by only 6 %.

For the contribution coming from disordered superconductor with $s$-wave pairing (Al), it is useful to recast the kinetic inductance per unit length in terms of the sheet resistance. To this end, we use the expression for penetration depth $\lambda$ via superfluid density $\rho_s$, $\lambda^2 = m/(\mu_0\rho_s e^2)$. In the Sec. IV A we express the $\rho_s$ via dimensionless superfluid density $n_s$ that is normalized to approach identity in the zero temperature and zero-field limit, as $\rho_s = n_s\rho_t$, see Eq. (S17). While the $\rho_t$ would coincide with the full density of carriers in the clean superconductor (denoted as $\rho_{\rm Al}$ ), presence of disorder leads to suppression that is proportional to the transport scattering time $\tau_{\rm tr}$ and zero-temperature and zero-field superconducting gap $\Delta_0$, resulting in the following value of $\rho_t = \rho_{\rm Al}\pi\Delta_0\tau_{\rm tr}/\hbar$. Substituting this into expression for kinetic sheet inductance we obtain:

$$L_{\square,\rm Al} = \frac{m}{\rho_s e^2 d} = \frac{\hbar m}{\rho_{\rm Al}\pi\Delta_0\tau_{\rm tr}e^2 d}\frac{1}{n_s} = \frac{\hbar}{\pi\Delta_0 d\sigma_{\rm Al}}\frac{1}{n_s}, \tag{S5}$$

where we used the Drude expression for conductivity of aluminum $\sigma_{\rm Al}$. From here, we convert the sheet inductances to inductances per unit length by multiplying $L_{\square,\rm Al}$ by the geometric factor $\gamma$:

$$L_{\rm Al} = \gamma\frac{\hbar R_{Al}}{\pi\Delta_0 n_s}, \tag{S6}$$

where $R_{\rm Al} = m/(\rho_{\rm Al}e^2\tau_{\rm tr}d)$ is the aluminum sheet resistance, $\Delta_0$ is zero-temperature and zero-field superconducting gap of Al, and the dimensionless superfluid density $n_s$ is given in Eq. (S17). This formula agrees with the commonly used expression [1].

For the semiclassical $p$-wave theory, which assumes a clean limit, the superfluid density reads $\rho_p = n_p\rho_{\rm InAs}$ where $\rho_{\rm InAs}$ is the two-dimensional density of carriers in InAs, and the normalized superfluid density $n_p$ is given by Eq. (S32). This results in a following contribution to inductance:

$$L_{\rm InAs} = \gamma\frac{m}{e^2\rho_{\rm InAs}}\frac{1}{n_p}. \tag{S7}$$

Note that this result is independent of film thickness because it is framed in terms of a two-dimensional density, $\rho_{\rm InAs}$. Using the equation for the kinetic frequency, $f_{\rm kin} = (2l\sqrt{L_{\rm kin}C})^{-1}$, where $l$ is the resonator length, and the fact that the inductances add in parallel, we obtain:

$$f_{\rm kin}^2 = \frac{1}{4l^2C}\left(L_{\rm Al}^{-1} + L_{\rm InAs}^{-1}\right) = \frac{1}{4l^2C\gamma}\left(\frac{\pi\Delta_0}{\hbar R_{\rm Al}}n_s + \frac{e^2\rho_{\rm InAs}}{m}n_p\right), \tag{S8}$$

where we made use of Eqs. (S6-S7). Collecting the all factors in front of $n_s$ and $n_p$, we arrive to Eq. (S2) with the following expression for constants $c_{s,p}$:

$$c_s = \frac{\pi^2\Delta_0}{2l^2C\gamma hR_{\rm Al}} \quad\text{and}\quad c_p = \frac{e^2\rho_{\rm InAs}}{4l^2C\gamma m}. \tag{S9}$$

### C. Analysis steps

In the main text we examine a so-called "null hypothesis", that corresponds to the absence of InAs layer. This situation is accounted for by setting $c_p = 0$, thereby turning Eqs. (S1)-(S2) into conventional pair-breaking theory for Al in presence of in-plane magnetic field. This model fits for a geometric resonant frequency and $c_p$, both of which give values similar to the full two-component model.

The analysis within the "full model" is divided into three following steps:

(i) Extracting $T_c(B)$ and $T_{c,0}$ from transport measurements on a co-fabricated device, as shown in Fig. 2(e) of the main text.

(ii) Simultaneous fit of $f_r(B=0,T)$ (Fig. 2(c)) and $f_r(B_x, T=0.1$ K) from Fig. 3(a) datasets using $f_{\rm geo}$, $c_s$, $c_p$, $B_x^*$ as fit parameters. Fit values and expectations are summarized in Table SI.

(iii) Fitting of second $g$-factor principal component, $g_y$, from a field-angle sweep.

In the final stage of fitting, the fit is restricted to regimes in which the theory is unconditionally stable, corresponding to angular differences of 45° from the $x$-axis.

We now summarize the four consistency checks on the four fit parameters obtained from the stage (ii) of the analysis, which are listed more briefly in Table SI.

1. To check the value of $f_{\rm geo}$, we perform a finite-element simulation and find 6.05 GHz, which is only 2% larger than the fit value.

2. To check $c_s$, we use expression from Eq. (S9) to calculate the sheet resistance of the Al, finding 6.7 Ω, in reasonable agreement with the separately-measured sheet resistance of other MBE grown Aluminum directly on InP of which gives values in the range 5 Ω. The resistance of such films can vary substantially over time due to oxidation, so it is also worthwhile to note that $c_s$ implies an aluminum resistivity of 10 μΩcm, reasonable for a high-quality Al 15 nm-thin film at low temperature.

3. To check $c_p$, we calculate the density using Eq. (S9) with $m = 0.04m_e$ [10], finding a density of $4 \times 10^{13}$ cm$^{-2}$. Because this density is extracted from a clean-limit formula which is likely not strictly valid for the InAs, we conservatively quote the density with a single digit of precision. This value is much larger than the density from Hall data measured for InAs without Al (Sec. III A), which is plausible due to the expected strong band-bending at the Al interface [11, 12]. Combining this density with the inferred Al sheet resistance and the measured transport device resistance yields a mobility $2 \times 10^4$ cm$^2$/(Vs), in agreement with the Hall data without Al (Sec. III A).

4. To check the value of $B_x^*$ we convert it to the $g$-factor using the value of Al gap of 217 μeV (determined from $T_c$), resulting in $g_x = 11.2 \pm 0.2$, in-line with values from 3-11 measured on similar quantum wells [7–10].

For the superfluid density, values of $f_{\rm geo}$, $c_p$, and $c_s$ are extracted from fit parameters. The inferred superfluid density for an experimentally measured $f_r$ is then given by inverting Eqs. (S1-S2),

$$n_p = \frac{1}{c_p}\left(\frac{1}{f_r^2} - \frac{1}{f_{\rm geo}^2}\right)^{-1} - \frac{c_s}{c_p} n_s, \tag{S10}$$

where $n_s$ is calculated numerically from Eq. S17.

## II. ADDITIONAL DATASETS

Here we present additional datasets. For the sample in the main text, we first show how the contribution to error bars accounting for hysteretic frequency shifts is derived, discuss in more detail the fit for $g_y$, and then examine an additional scenario of a hypothetical 2DEG with large $g$-factor but no spin-orbit coupling. This is conceptually useful for understanding how our technique detects the breakdown of $p \pm ip$ pairing.

| Parameter | Fit value | Consistency test |
|---|---|---|
| $f_{\rm geo}$ | $5.95 \pm 0.01$ GHz | Agrees within 2% with value from finite-element model |
| $c_s$ | $78 \pm 2$ GHz$^2$ | Implies Al sheet resistance of 6.7 Ω, which agrees with measured sheet resistance of MBE-grown Al of 5 Ω. |
| $c_p$ | $143 \pm 6$ GHz$^2$ | Implies InAs mobility $\mu = 2 \times 10^4$ cm$^2$/(V · s), in agreement with Hall measurements in Sec. III A. |
| $B_x^*$ | $333 \pm 2$ mT | Implies $g$-factor $g_x = 11.2 \pm 0.1$, this is within the range of 3-11 previously measured in similar InAs quantum wells [7–9]. |

Table SI: Summary of all fit parameters from the stage (ii) of analysis. There are four consistency tests for the four fit parameters, that are discussed in Sec. I C in greater detail.

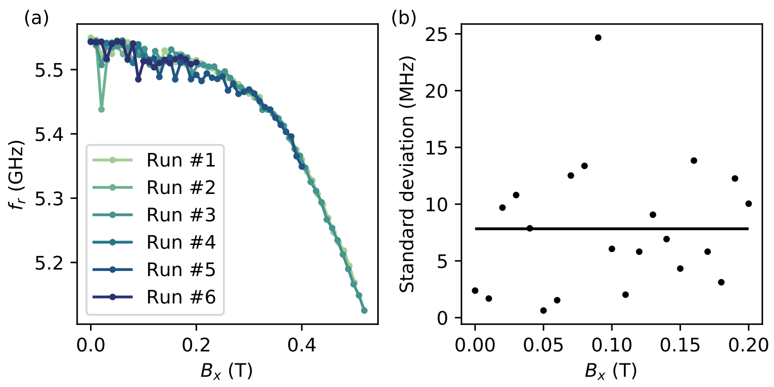


Figure S2: (a) Repeated measurements of $f_r$ vs $B_x$. (b) Standard deviation at each frequency point. Horizontal line is at the average value of 7.8 MHz, which is added in quadrature to all $f_r$ points in the main text.

Then we introduce new samples fabricated on rotated crystal axes, showing that the anisotropy of the resonant frequency is also rotated. This shows experimentally that the origin of the anisotropy is the crystal. With one of these samples, we then show additional studies of power dependence and the effect of magnetic-field misalignment.

### A. Error estimates

All $f_r$ error bars in the main text include error from hysteretic frequency shifts associated with imperfect magnetic-field compensation. To quantify these shifts, we have repeated several sweeps of the data in Fig. 3a and computed a standard deviation [Fig. S2(a)]. We compute an average error associated with hysteretic frequency shifts [Fig. S2(b)], and add it in quadrature with the standard error for each frequency value.

### B. Effect of reduced induced gap

In our analysis we make the simple assumption that the induced gap is equal to the Al gap, $\Delta = \Delta_{\rm Al}$. We have checked if this assumption is reasonable by performing SNS tunneling spectroscopy on a sister wafer, which measures the induced gap at the edge of the Al/InAs heterostructure. Considering this as a lower bound, we find $\Delta > 0.83\Delta_{\rm Al}$. To assess if this could have a substantial impact on our analysis, we have re-analyzed the data assuming a worst-case induced gap of $0.83\Delta_{\rm Al}$, and found an InAs density of $1.5 \times 10^{14}$ cm$^{-2}$, mobility of $1 \times 10^4$ cm$^2$/(Vs) and $g$-factor of 9. We conclude that, even assuming a worst case for induced gap, our results are not strongly affected.

### C. Fit for $g_y$

In the main text we quote the best-fit value of $g_y = 4$. To avoid including potentially unstable regions in fitting, we have included only unconditionally stable regions in a fit to the angle-dependence, corresponding to the non-shaded angles in Fig. 4 in the main text. The result of the fit for $g_y$ is unusual because there is no local minimum for $g_y$ as a fit parameter [Fig. S3]. Rather, $\chi^2$ saturates for $B_y^* > 0.91$ T, corresponding to $g_y < 4$. The physical interpretation of this behavior is that for $g_y < 4$ one is in the regime $B_y^* < B_{c,\rm Al}$, where $B_{c,\rm Al}$ is the critical field of the aluminum field. In this regime the Al goes normal before the InAs enters into a gapless phase, and thus one can only bound the $g$-factor. Based on constraints from the expected $g$-factor anisotropy of our asymmetric (100) quantum well, and known $g$-factors in similar quantum wells, we choose to plot the physically reasonable value $g_y = 4$ in the main text.

### D. Effect of spin-orbit coupling

To better understand the role of spin-orbit coupling on the combined model for superfluid density, it is useful to consider a hypothetical system with a large $g$-factor and no spin-orbit coupling. In this case Pauli pair-breaking is dominant, and one physically expects the superconducting gap to close uniformly in momentum space. Similar to

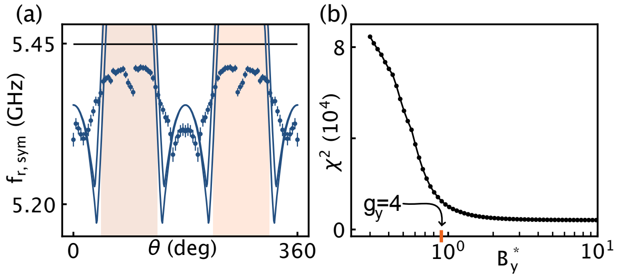


Figure S3: (a) Same as Fig.4(c) in the main text but showing two theory curves. Measured $f_r$ at $|B| = 0.4$ T symmetrized about $\theta = 180°$. Black curve is prediction of the $s$-wave pair-breaking theory. Upper blue curve is $g_y = 0$, lower blue curve is $g_y = 4$. For $g_y < 4$ the theory curves are hardly effected. (b) Goodness of fit $\chi^2$ versus $B^*_y$, which is related to $g_y$ by $g_y \mu_B B^*_y = \Delta$. $\chi^2$ does not have any local minima, but rather saturates for $B^*_y > 0.91$ T, corresponding to $g_y < 4$.

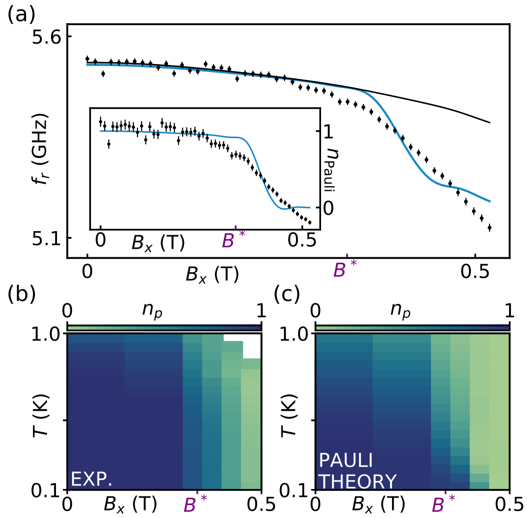


Figure S4: Fit to data without spin-orbit coupling included in the 2DEG (Pauli pair-breaking only). (a) Resonant frequency $f_r$ as a function of $B_x$. Black is curve is orbital pair-breaking theory with no free parameters, blue line is a fit to a theory that includes only Pauli pair-breaking in the 2DEG. Inset: Inferred superfluid density in the 2DEG, compared with the Pauli-only theory. The Pauli-only theory predicts more abrupt suppression of superfluid density with magnetic field, compared to what is observed in the experiment. (b) Experimental phase diagram of the inferred superfluid density in the 2DEG. (c) Theoretical phase diagram of the Pauli-suppressed superfluid density. In the absence of spin-orbit coupling, much stronger temperature dependence of Pauli-suppressed superfluid density is expected due to the participation of the entire Fermi surface.

the $p$-wave theory, this situation is known to drive an instability, which in a single-component system results in an FFLO [13, 14] state for a narrow range of magnetic fields. Motivated by the fact that superconductivity is proximity-induced by aluminum, which will create a large energy penalty for the FFLO state, here we ignore these effects and proceed with the superfluid density expressions given in Sec. IV B 4.

In this section, we refit to our two-fluid expression, Eq. (S2) to the such "Pauli-suppressed" model. The results are shown in Fig. S4. The best-fit predicts a much sharper decrease in frequency with magnetic field, compared to the one observed in the experiment. Physically this is due to the fact that the gap closes abruptly instead of in isolated regions in momentum space. Further, the temperature dependence is much stronger in this "Pauli-suppressed" coupling scenario, again due to the fact that the suppression of pairing is uniform across the entire Fermi surface.

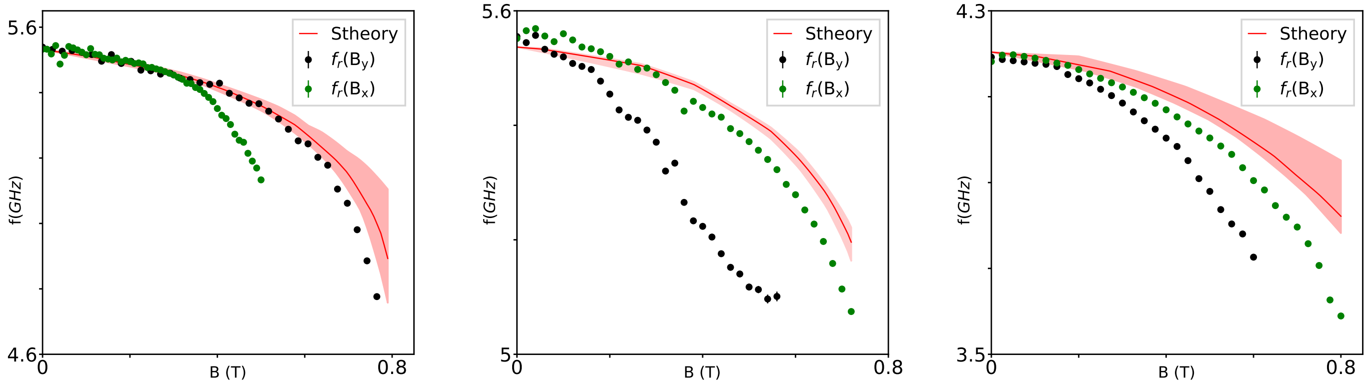


(a) Sample A (b) Sample B (c) Sample C

Figure S5: Resonance frequency plotted as a function of $x$- and $y$-oriented magnetic field with s-wave superconductivity model (red line). Uncertainty band of the theory curve is calculated using the upper/lower resistance threshold for extracting $T_c(B)/T_{c0}$.

## E. Crystal orientation tunes anisotropy

We present in this section the study of field-dependence across three samples, labelled Samples A, B, and C, with Sample A corresponding to the sample that is more widely discussed in the main text of the article. The devices in Samples B and C are rotated by 90° with respect to the crystal axes compared to Sample A. This tests the key hypothesis in the main text that the anisotropy in resonant frequency is set by the crystal axes due to the $g$-factor.

Figure S5 shows the shift in measured resonant frequency across the three samples, as a function of magnetic field, with green points showing the field evolution in the $x$-axis, and black points showing the field evolution in the $y$-axis. The red curve followed the $s$-model ($c_p$=0) presented in the main text and discussed in Sec. I above.

Comparing Figures S5a and S5b, we can observe that the deviation in frequency shift from the $s$-theory switch occurs in the $x$-direction for Sample A, but for the $y$-field direction Samples B and C. This is the expected behavior due to the fact that anisotropy is dominated by the $g$-factor, which is locked to the crystal axes.

This effect is more clear when we look at the angle plot in Figure S6, which appears perpendicular in orientation to that of Sample A, presented in Fig. 4 of the main text. Interestingly, no minor lobes are observed in the angle plot. Although we cannot make a firm comparison with theory for these samples due to the dominance of the instability for this device orientation, the lack of minor lobes is qualitatively consistent with the fact that, for the rotated samples,

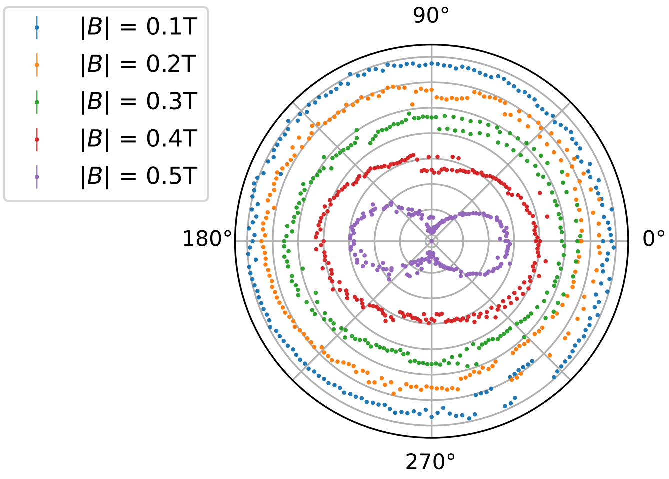


Figure S6: Sample C: Measured resonant frequency at different field magnitudes and orientations. Radial increment is 50 MHz.

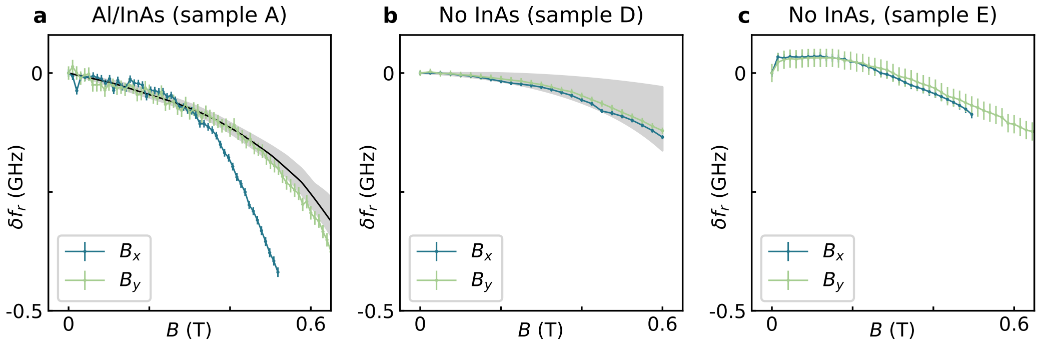


Figure S7: Comparison of samples with and without InAs heterostructure. Each subfigure shows the filed-induced frequency shift, $\delta f_r$ as a function of field for both the $x$-direction ($B_x$) and $y$-direction ($B_y$). (a) Sample with InAs from main text. For this sample $f_r(B=0) \sim 5.5$ GHz. Grey band shows $s$-wave pair-breaking theory with no free parameters accounting for systematic uncertainty in transport-extracted $T_c(B)$ due to nonzero width of superconducting transition, black line shows curve from main text. (b) Sample without InAs. For this sample $f_r(B=0) \sim 5.4$ GHz. Grey band shows $s$-wave pair-breaking theory with no free parameters accounting for systematic uncertainty in $T_c(B)$. In this sample different runs gave unusually large difference in $T_c(B)$, which is not understood. (c) Another sample without InAs. For this sample $f_r(B=0) \approx 5.3$ GHz.

increasing the field angle both moves the Fermi arcs parallel to the dominant resonator direction and increases the $g$-factor. Both of these effects decrease superfluid density. In contrast, in the sample in the main text, rotating the field causes a competition between rotating the Fermi arcs and *decreasing* the $g$-factor.

## F. InAs heterostructure causes anisotropy

As a control experiment, we have measured several samples with Al grown directly on the InP substrate [Fig. S7]. Repeating the measurement and alignment procedure discussed in the main text on samples without InAs, we find that there is negligible magnetic-field anisotropy. This observation rules out a large class of trivial explanations for our observations such as vortices due to imperfect field-alignment. To easily compare across devices and remove small hysteretic shifts, we have reported the field-induced frequency shift, $\delta f_r(B) = f_r(B) - f_r(B=0)$. Magnetic-field alignment in Al-only sample E was especially challenging, which is not understood. Larger error bars on this sample reflect this challenge.

## G. InAs heterostructure causes abrupt increase in dissipation

To further strengthen the observation of an abrupt increase in dissipation at $B^*$ presented in Fig. 5 of the main text, we emphasize that such behavior is not generically observed for superconducting resonators. For instance Fig. S8(a) shows that the abrupt increase in dissipation disappears when InAs is removed. For completeness, we also present linecuts of Fig. 5 in the main text separately in Fig S8(b).

## H. Power dependence of the resonant frequency and quality factor

A few input power sweeps at different magnetic fields have been done to ensure that our results are not altered by input-power dependence of the resonance. Two typical datasets measured at the in-plane magnetic fields of 0 T and 0.35T are shown in Fig. S9. All powers are reference to the sample only accounting for attenuation from manually placed attenuators. This neglects the effect of the stainless-steel coaxial cables inside the cryostat (measured 10 dB insertion loss at room temperature), and the room-temperature cables outside of the cryostat (nominal 6 dB insertion loss). The quoted powers are therefore very conservative, and realistically overestimate the true power at the sample by at least 10 dB.

When the magnetic field is zero, the resonant frequency and quality factor are stable and insensitive to the input power from $-130$ dBm to $-80$ dBm as they are shown in Fig. S9(a),(c). At $B_x$=0.35 T the resonant frequency

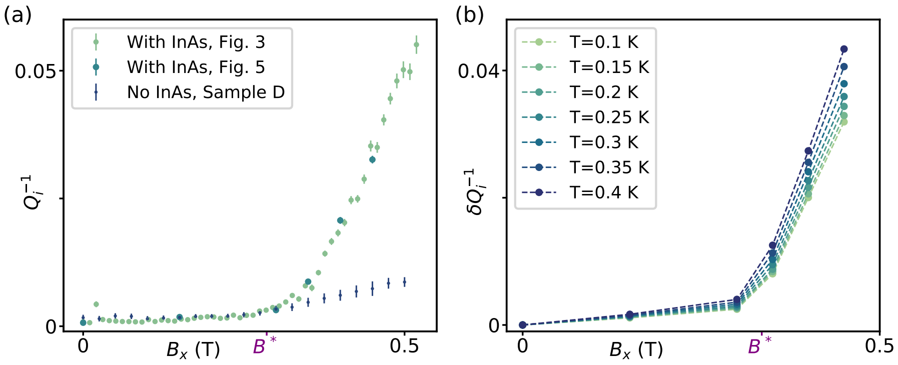


Figure S8: (a) Resonator dissipation, measured by inverse intrinsic quality factor $Q_i^{-1}$ as a function of magnetic field $B_x$ for different datasets. (b) Linecuts of excess resonator dissipation, $\delta Q_i^{-1}$, from Fig. 5 in the main text.

and quality factor have a barely resolvable power dependence (Fig. S9(b),(d)). Specifically, at an input power of $> -80\,\mathrm{dBm}$, the resonant frequency drops by less than $2\,\mathrm{MHz}$. Although this power independence is interesting in its own right, it is negligible on the scale of the effects we have observed in the main text. For a sense of scale, the typical error bars due to hysteretic effects in our measurements in the main text are $5-10$ MHz, and the overall scale of the effects we observe are 500 MHz. In the main text, all data are taken at a $-85\,\mathrm{dBm}$ level, ensuring that power-dependent effects have a negligible contribution to the data. During data acquisition we periodically, manually checked for power dependence by manually lowering the VNA power, often down to the single-photon level, and did not observe any significant changes.

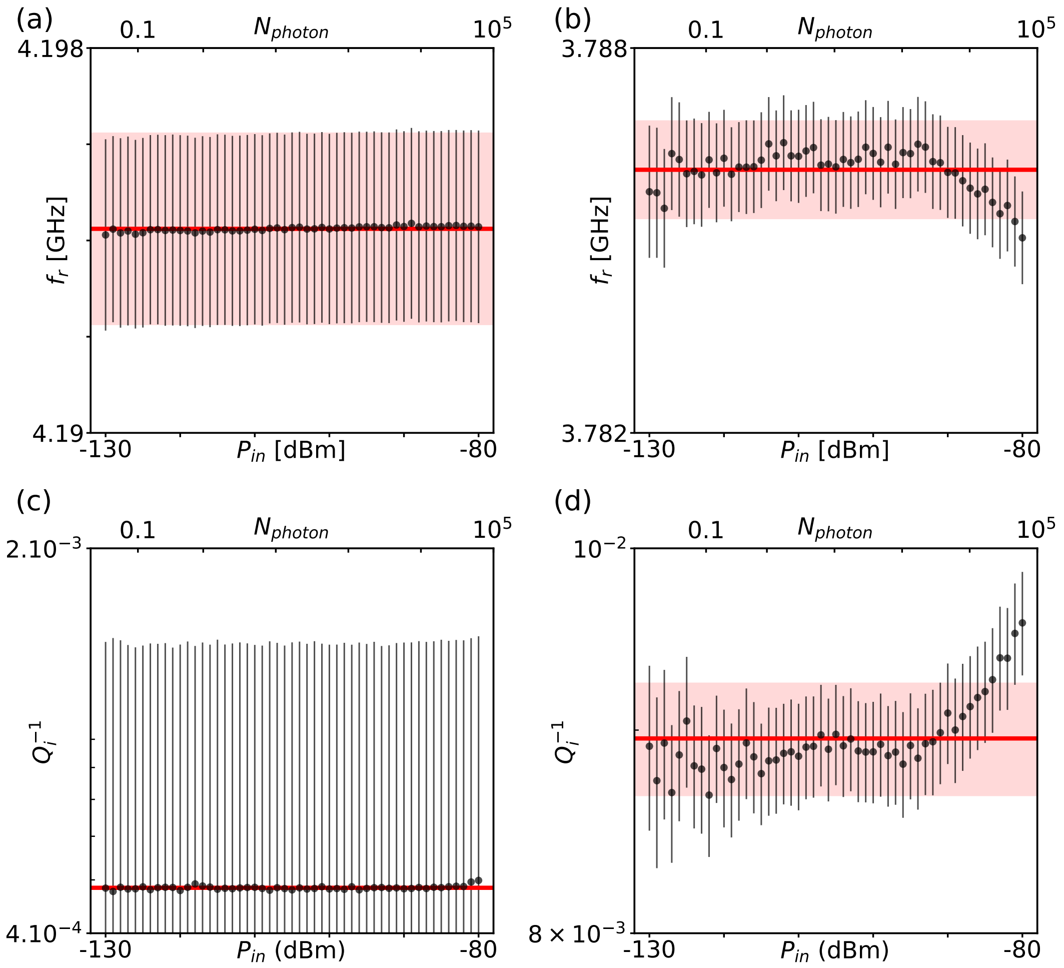


Figure S9: Sample C: Resonance frequency and inverse quality factor from power sweeps at $B_x = 0$ T (a,c) and $B_x = 0.35T$ (b,d). Error bars in this plot are standard errors from the fit parameters.

### I. Line cuts of $n_p(B,T)$

To aid in comparison of theory an experiment, here we present line cuts of the data in Fig. 3(b,c) in the main text in Fig. S10. There is good agreement with theory. We emphasize that these theoretical curves have no free parameters.

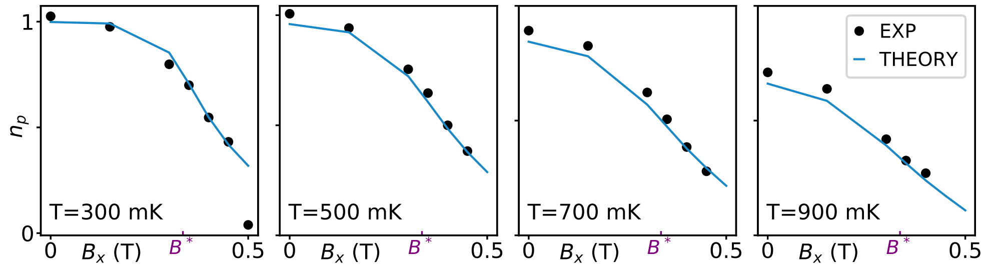


Figure S10: Comparison of $n_p$ from experimental measurement (black dot) and theoretical model (blue curve) as a function of magnetic field for different temperatures. Data are from Fig. 3(b,c) in the main text.

### J. Cartesian field-angle plots

To assist readers in comparing the experimental field-angle dependence of the resonator frequency with the $p \pm ip$ model we provide a plot similar to Fig. 4 in the main text, but in a Cartesian plane [Fig. S11]. Although there is qualitative agreement, theory predicts stronger angular variations than are observed in experiment, which we attribute to the role of the instability.

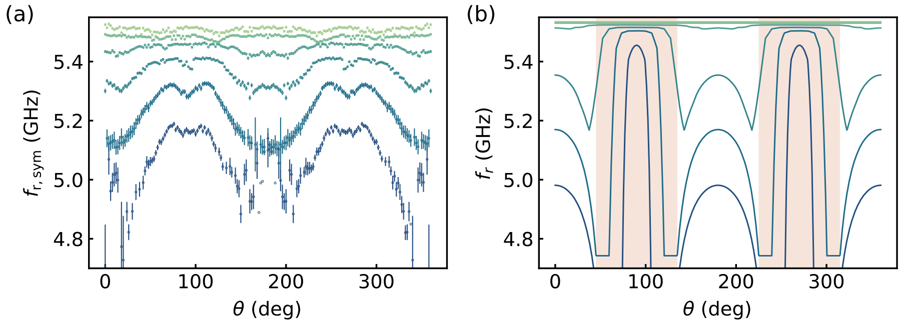


Figure S11: (a) Symmetrized resonant frequency, $f_{\rm r,sym}$ measured as a function of field angle $\theta$. (b) Theoretical prediction for $f_r(\theta)$.

## III. FURTHER EXPERIMENTAL INFORMATION

### A. Material Growth

As shown in Fig. S12, the samples were grown on a semi-insulating InP (100) substrate, using a modified Gen II molecular beam epitaxy system. A buffer layer of graded $In_xAl_{1-x}As$ is grown on the substrate at low temperature to help mitigate formation of dislocations originating from the lattice mismatch with the InP substrate. The indium content of $In_xAl_{1-x}As$ is step-graded from $x = 0.52$ to 0.81 in steps of $\Delta x = 0.02$ every $\approx 50$ nm. Next, a delta-doped Si layer of $\approx 1$ x $10^{12}$ cm$^{-2}$ density is placed here followed by 6 nm of $In_{.81}Al_{.19}As$. The quantum well is grown next, consisting of a 4 nm thick layer of $In_{0.81}Ga_{0.19}As$ layer, a 7 nm thick layer of InAs, and finally a 10 nm thick top layer of $In_{0.81}Ga_{0.19}As$. In order to deposit Al layer-by-layer, the substrate is cooled to sub-zero temperatures to promote the growth of Al (111). The transport properties of the wafer are characterized in a van der Pauw geometry at T =

1.5 K. The density and mobility are determined to be $n \approx 1.07 \times 10^{12}$ cm$^{-2}$ and $\mu_e \approx 12750$ cm$^2$/Vs which lead us to an electron mean free path of $\approx 217$ nm.

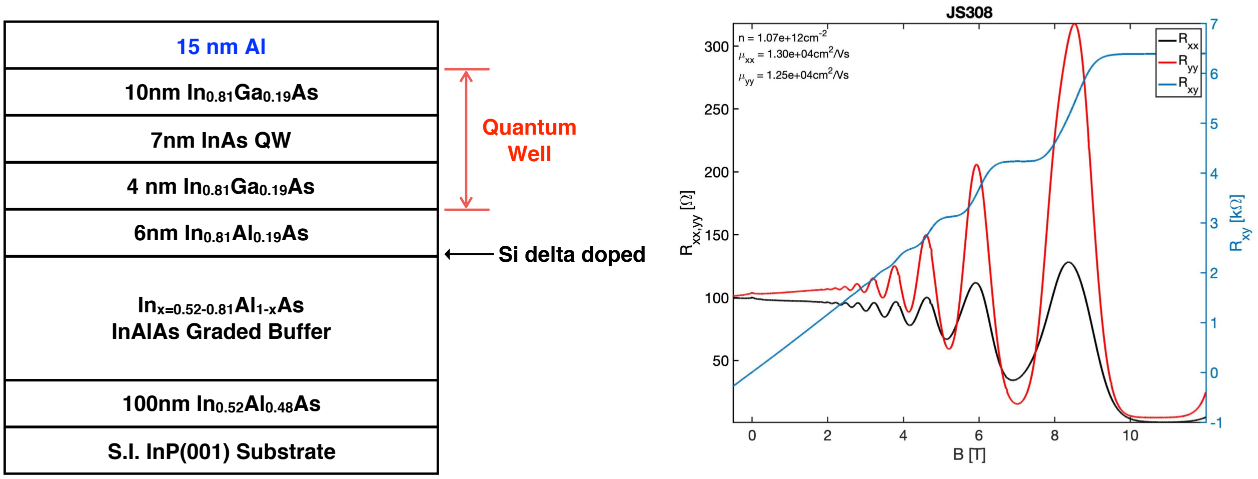


Figure S12: (left) Schematic of growth stack. (right) Resistance vs magnetic field for InAs material.

## B. Magnetic field alignment

To ensure the absence of orbital contributions, perpendicular magnetic-field components are canceled at each applied parallel field by minimizing the on-resonant transmission. This metric is extremely sensitive to misalignments – we estimate that, for a parallel field of 1 T, the residual out-of-plane component is comparable to Earth's magnetic field. To conservatively include the effect of small alignment errors on the data, error bars cover the range of hysteretic shifts in a repeated dataset for all measured $f_r$ (see Supplement). We have noticed that, even with our best alignment procedures, residual hysteretic behavior is larger in some device than others. Better controlling and ultimately eliminating such effects will be important for further development of this technique.

To experimentally explore the effect of misalignment on the anisotropy we have observed, we have intentionally misaligned the magnetic field and repeated the measurements in the main text. Finding the optimal perpendicular compensation field for each applied $x$ and $y$ field generates two lines (Fig. S13(b,c)), which is the expected behavior for a slightly tilted sample. Once the slope of these two lines is known an aligned field can be generated at any angle in the chip plane from straightforward trigonometry. Fig. S13(a) shows three angle sweeps at field magnitude of 0.5 T with different field alignments: optimum alignment (in black), single-axis misalignment (in blue), and two-axis misalignment (in red). This optimum alignment results in the highest frequencies, and an anisotropy aligned with the $x - y$ axes. Single-axis misalignment causes a slight tilt, and two-axis misalignment shows severely suppressed frequencies with a large tilt. Points from misaligned curves fall within those from the aligned curves to within the experimental scatter, indicating that our field alignment is correct.

## C. Sample Fabrication

The quantum well consists of a 7 nm InAs layer on a buffer stack epitaxially grown on an InP (100) wafer. An intermediate 10 nm InGaAs layer is then grown on top, before the structure is capped by a 15 nm epitaxial aluminum thin film. Without aluminum, the semiconductor has a Hall mobility $\mu = 1.3 \times 10^4$ cm$^2$/(Vs) and density $n = 1.06 \times 10^{12}$ cm$^{-2}$. Measurements on the transport device give the Al critical temperature $T_c(0) = 1.43$ K, a typical value for Al thin films [15], and a parallel critical field of approximately 0.91 T. The sample mask made by spinning PMMA 600K resist is patterned using a Raith EBPG5150 electron-beam lithography system. The mask is then developed in an IPA 7:3 DI water solution. To form the mesas and transport devices, excess of epitaxial Al layer has been removed by a wet etch with Transene D at 50°C. The semiconductor stack is subsequently etched using an H2O2:H3PO4:Citric acid mixture. The ground plane and transmission line structures are grown by physical vapor deposition of of 5 nm Ti/50 nm Nb in a Plassys MB UHV system, with excess material removed by lift-off in acetone. The center pin width and the spacing to the ground plane of the resonator are 25 $\mu$m and 16 $\mu$m, respectively. The

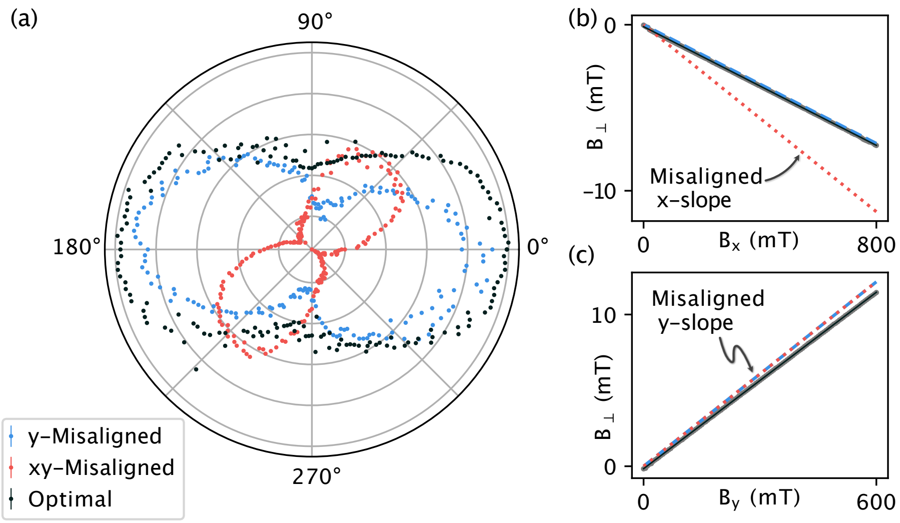


Figure S13: Sample C: Effect of misalignment on the angle sweep curve shapes. (a) Resonant frequency as a function of magnetic-field angle for three different alignments. Black points represent optimal alignment (corresponding to black curves in (b,c)), blue points represent single-axis misalignment (corresponding to blue curves in (b,c)), red-points represent two-axis misalignment (corresponding to red curves in (b,c)). (b,c) Applied perpendicular field for applied field in the $x$-direction (b) and $y$-direction (c). Black curves are the optimum determined by minimizing resonant transmission at each point, with slopes of $(-8935 \pm 5) \times 10^{-6}$ for $x$-direction and $(19383 \pm 6) \times 10^{-6}$ in $y$-direction. Blue curves have single-axis misalignment in the $y$-direction, with a slope of $20.257 \times 10^{-3}$. Red curves have a $y$-axis misalignment the same as blue, but an additional $x$-axis misalignment of $-14.079 \times 10^{-3}$.

length of the resonator is 9337 mm. These geometric parameters are selected for an impedance of 50 Ω and a geometric resonant frequency of 6.07 GHz.

## IV. THEORY FOR SUPERFLUID DENSITY AND DISSIPATION

### A. Depairing theory of aluminum superconductivity

In order to understand the additional contribution of InAs in the electromagnetic response of the system, we discuss first the contribution of Al thin film. Since the Al is expected to be a dirty superconductor with standard s-wave pairing, we review the theory required for fitting experimental results. In particular, we are interested in extracting the effect of in-plane magnetic field on the self-consistent gap in Al which will be used later for calculating electromagnetic response of InAs. In the following theory discussion we have used Gaussian units. Since in the fitting procedure only results for dimensionless quantities are used, this does not cause any problem.

The depairing mechanism due to the time-reversal symmetry breaking perturbations was first considered by the Abrikosov and Gorkov [16] for magnetic impurities and later extended to other mechanisms [17]. In a dirty limit there is a universal relation to determine the dependence of the critical temperature on pair-breaking parameter, namely

$$\ln\left(\frac{T_c}{T_{c0}}\right) + \psi\left(\frac{1}{2} + \frac{\alpha}{2\pi k_B T_c}\right) - \psi\left(\frac{1}{2}\right) = 0, \tag{S11}$$

where $T_c$ is the critical temperature ($T_{c0}$ in the absence of perturbation), $\psi(x)$ is the so-called digamma function (logarithmic derivative of the gamma function) and $\alpha$ is the pair-breaking parameter. Generally $\alpha \propto \tau\langle(\delta H)^2\rangle$, where $\tau$ is the characteristic "ergodization" time (will be defined more precisely below as transport scattering time) and $\delta H$ is the time-reversal symmetry breaking part of the Hamiltonian that will be proportional to in-plane magnetic field in our case [18]. We assume the limit of strong disorder that implies that "ergodization" process (given by the elastic impurity scattering) occurs on the length scales shorter than coherence length. This corresponds to condition $\tau\Delta/\hbar \ll 1$, where $\Delta$ is the order parameter. Since we are interested in magnetic field dependence of the critical temperature, we will concentrate on two mechanisms of time-reversal symmetry breaking: orbital effects for thin film in parallel magnetic field and Pauli paramagnetism due to exchange fields.

For the pair-breaking due to orbital effects, the notion of the thin film and order parameter being constant over the sample require $d \ll (l\xi_0)^{1/2}$ and $d \ll \lambda$, where $d$ is the thickness of the sample, $l$ is the mean free path, $\xi_0$ is the superconducting coherence length and $\lambda$ is the penetration depth. The pair-breaking parameter depends on the relation between mean free path and thickness of the film. If mean free path is short, $l \ll d$, corresponding to diffusive motion on the scale of $d$, the pair-breaking parameter reads [18]:

$$\alpha_{\mathrm{tr}} = \frac{\tau_{\mathrm{tr}} v_F^2}{18\hbar c^2} (eHd)^2 = \frac{D}{6\hbar c^2} (eHd)^2 , \tag{S12}$$

where $\tau_{\mathrm{tr}}$ is the transport collision time, which is related to diffusion constant $D = v_F^2 \tau_{\mathrm{tr}}/3$. In the more general case $\alpha = \frac{\tau_{\mathrm{tr}} v_F^2}{18\hbar c^2} (eHd)^2 g\left(\frac{\pi l}{d}\right)$, where $g(x) = \left(3/2x^3\right)\left[\left(1+x^2\right)\arctan x - x\right] \approx 3\pi/4x$ for $x \gg 1$. This reduces to the following expression in the ballistic regime, $l \gg d$ [19]:

$$\alpha_{\mathrm{b}} = \frac{v_F d^3}{24\hbar c^2} (eH)^2 . \tag{S13}$$

For the case when pair-breaking originates from the Pauli paramagnetism, the pair breaking parameter reads [20]:

$$\alpha_{\mathrm{so}} = \frac{3\tau_{\mathrm{so}} e^2 \hbar H^2}{8m^2c^2}, \tag{S14}$$

where $\tau_{\mathrm{so}}$ is the characteristic spin flip scattering time due to spin-orbit coupling. Since spin-orbit coupling is expected to be small in Al, we expect the first mechanism to dominate. Crucially, for both mechanisms the pair-breaking parameter depends quadratically on magnetic field strength $\alpha = \alpha_0 + H^2/H_0^2$, where $\alpha_0$ accounts for mechanisms of pair-breaking which do not depend on magnetic field, such as magnetic impurities. The remarkable aspect is the universality of pair-breaking theory in the strong disorder case, which allows one to avoid discussion of the microscopic source of pair breaking and convert the measured $T_c(B)$ into pair-breaking parameter $\alpha$ using Eq. (S11).

Once the pair-breaking parameter is known it can be used to obtain the superconducting gap in Al self-consistently. Considering the Green's function in the presence of impurity scattering and magnetic field we get [17]:

$$\frac{\omega_n}{\Delta} = u_n \left(1 - \frac{\alpha}{\Delta\sqrt{1+u_n^2}}\right), \tag{S15}$$

where $\omega_n = 2\pi\,(n+1/2)\,k_B T$ are the Matsubara frequencies and $u_n = \tilde{\omega}_n/\tilde{\Delta}$, $\tilde{\omega}_n$ and $\tilde{\Delta}$ being renormalized frequency and order parameter. Determining $u_n$ from (S15) and substituting into self-consistency equation for the order parameter [17], we get:

$$\Delta \ln\left(\frac{T}{T_{c0}}\right) = 2\pi k_B T \sum_{n>0} \left(f_n - \frac{\Delta}{\omega_n}\right), \tag{S16}$$

where $f_n = 1/\sqrt{1+u_n^2}$ and we obtain $\Delta$ as a function of $H$. This dependence $\Delta(H)$ is then used in the following section to study the electromagnetic response of InAs layer.

Finally, after determining the self-consistent gap, the superfluid density in Al is calculated as [18]

$$n_s = \frac{\rho_s}{\rho_t} = \frac{\hbar}{\pi\tau_{\mathrm{tr}}\Delta_0} \sum_n \frac{\pi k_B T f_n^2}{\frac{\Delta}{f_n} + \frac{\hbar}{2\tau_-}} \approx \frac{k_B T}{\Delta_0} \sum_n \frac{f_n^2}{\frac{\tau_{\mathrm{tr}}\Delta}{\hbar f_n} + \frac{1}{2}} \tag{S17}$$

where $n_s$ is the dimensionless fraction of carriers participating in the condensate, normalized to assume values between 1 and 0, $1/\tau_- = 1/\tau_{\mathrm{tr}} - \alpha \approx 1/\tau_{\mathrm{tr}}$ (since $1/\tau_{\mathrm{tr}} \gg \alpha$) and $\Delta_0$ is the value of gap at $T=0$ and in absence of pair breaking. This choice of normalization of $n_s$ leads to the following value of $\rho_t = \rho_{\mathrm{Al}}\pi\tau_{\mathrm{tr}}\Delta_0/\hbar$, that accounts for suppression of superfluid density at zero field and zero temperature due to disorder.

We note that our choice of normalization of $n_s$ assumes limit of strong disorder thus Eq. (S17) is practically independent of precise value of $\tau_{\mathrm{tr}}$ as soon as $\tau_{\mathrm{tr}}\Delta/\hbar \ll 1$. Our Al film has $\tau_{\mathrm{tr}}\Delta/\hbar \sim 10^{-3}$, placing it well in the disordered limit of the pair-breaking theory, where we have taken the transport scattering time taken to be 5 fs from the inferred Al sheet resistance and a nominal density of $10^{29}$ m$^{-3}$.

In the absence of pair breaking, $\alpha = 0$, Eq. (S15) gives $u_n = \omega_n/\Delta$, and in the dirty limit (corresponding to $\Delta/f_n \ll \hbar/2\tau_{\mathrm{tr}}$) the equation (S17) reduces to the well-known result $n_s = \tanh(\Delta/2T)$ that is by construction normalized to take values between zero and 1. Converting to conventional density we recover $\rho_s = \rho_{\mathrm{Al}}\,(\pi\tau_{\mathrm{tr}}\Delta/\hbar)\tanh(\Delta/2k_BT)$ — the standard expression for the superfluid density of disordered superconductors.

### B. Superfluid density in p-wave superconductor

#### 1. *Model for InAs*

The starting system Hamiltonian for InAs has the form

$$H(\mathbf{k}) = \sum_{\mathbf{k}} c_{\mathbf{k}}^{\dagger} \left[ \frac{\hbar^2 k^2}{2m} - \mu + \lambda_{so} \left( k_x \sigma^y - k_y \sigma^x \right) - V \sigma^y \right] c_{\mathbf{k}} + \Delta \left[ c_{\mathbf{k}\uparrow}^{\dagger} c_{-\mathbf{k}\downarrow}^{\dagger} + \text{H.c} \right], \tag{S18}$$

where $c_{\mathbf{k}}^{\dagger} = \left( c_{\mathbf{k}\uparrow}^{\dagger}, c_{\mathbf{k}\downarrow}^{\dagger} \right)$ is an electron creation operator with momentum $\mathbf{k}$ and spin $s = \uparrow$ or $s = \downarrow$, $m$ is the effective mass, $\lambda_{so}$ spin-orbit coupling strength taken to be constant and independent of other parameters such as disorder strength etc., $\mu$ chemical potential, $\Delta$ proximity s-wave superconducting order parameter due to Al and $V$-Zeeman field in $y$-direction

$$V = g\mu_B B, \tag{S19}$$

where $g$ is the $g$-factor in the corresponding direction and $\mu_B$ is the Bohr magneton. In order to calculate the electromagnetic response we need to obtain the Nambu Green's function $G(i\omega_n, \mathbf{k}) = (i\omega_n - H(\mathbf{k}))^{-1}$. For general case this can be done numerically. To obtain analytical insight we will resort to the limit $\mu \gg \Delta, V$ (this limit will be justified below) and decouple the two bands through definition of new operators [21]:

$$f_{\mathbf{k}}^{\dagger} = \left( c_{\mathbf{k}\uparrow}^{\dagger} + i e^{i\theta_{\mathbf{k}}} c_{\mathbf{k}\downarrow}^{\dagger} \right) / \sqrt{2}, \tag{S20}$$

$$d_{\mathbf{k}}^{\dagger} = \left( c_{\mathbf{k}\uparrow}^{\dagger} - i e^{i\theta_{\mathbf{k}}} c_{\mathbf{k}\downarrow}^{\dagger} \right) / \sqrt{2}. \tag{S21}$$

where $e^{i\theta_{\mathbf{k}}} = (k_x + i k_y) / |\mathbf{k}|$ and ignoring the terms which couple between bands. In the Nambu basis $F_{\mathbf{k}}^{\dagger} = \left( f_{\mathbf{k}}^{\dagger}, f_{-\mathbf{k}} \right)$, $D_{\mathbf{k}}^{\dagger} = \left( d_{\mathbf{k}}^{\dagger}, d_{-\mathbf{k}} \right)$ we get

$$\tilde{H}(\mathbf{k}) = \epsilon_{\mathbf{k}} \tau^z \pm \Delta \left( \sin\theta_{\mathbf{k}} \tau^x - \cos\theta_{\mathbf{k}} \tau^y \right) \mp \frac{V k_x}{k}, \tag{S22}$$

with $\epsilon_{\mathbf{k}} = \hbar^2 k^2 / 2m \pm \lambda_{so} k - \mu$, where $+$ $(-)$ corresponds to $F_{\mathbf{k}}^{\dagger}$ $(D_{\mathbf{k}}^{\dagger})$. Then the excitation spectrum will be

$$E_{\mathbf{k}}^{\mp,\pm} = \mp \frac{V k_x}{k} \pm \sqrt{\epsilon_{\mathbf{k}}^2 + \Delta^2} = \mp \frac{V k_x}{k} \pm \xi_{\mathbf{k}}, \tag{S23}$$

where first superscript corresponds to different bands and second to electron-hole excitation. Finally the Green's function is

$$G(i\omega_n, \mathbf{k}) = -\frac{\hbar \left[ \left( i\hbar\omega_n \pm \frac{V k_x}{k} \right) + \epsilon_{\mathbf{k}} \tau^z \pm \Delta \left( \sin\theta_{\mathbf{k}} \tau^x - \cos\theta_{\mathbf{k}} \tau^y \right) \right]}{\left( \hbar\omega_n \mp i \frac{V k_x}{k} \right)^2 + \xi_{\mathbf{k}}^2}. \tag{S24}$$

#### 2. *Bogoliubov Fermi surfaces*

As was discussed previously [21], with the inclusion of the Zeeman field the Hamiltonian (S18) can support gapless Bogoliubov excitations. With the increase of $V$ the quasiparticle spectrum tilts and banana-shaped Bogoliubov Fermi surfaces emerge as $V > \Delta$. This is demonstrated in Fig. S14 where the evolution of Fermi surfaces is shown as a function of $V$. We chose the parameters of the system comparable to the experimentally measured values, namely $\hbar^2/(2m\lambda_F^2) = 150\Delta$ and $\lambda_{so}/\lambda_F = 5\Delta$ (corresponding to the spin-orbit coupling strength of $\lambda_{so} = 100\,\text{meV} \cdot \text{Å}$), where $\lambda_F$ is the Fermi wavelength which is equal to 5.6 nm for the density determined in Sec. I C. The regime when Bogoliubov Fermi surfaces emerge has an important effect on superfluid density of the system, which will be discussed in the next section.

Fig. S15 shows the evolution of Bogoliubov Fermi surfaces with the change of the chemical potential $\mu$. The figure also compares the solutions obtained from Eq. (S18) and Eq. (S22). It is clear that when $\mu \gg \Delta$ the model that assumes two decoupled bands presented in the previous section is nearly identical with the solution of the original Hamiltonian Eq. (S18).

### 3. *Electromagnetic response of InAs layer*

In this section we calculate the electromagnetic response of InAs 2D layer in linear regime. We assume that InAs is a clean proximity-induced superconductor and disregard the impurity scattering. The current induced in the system due to the varying electromagnetic field can be written in usual form [17]

$$j_{\mu}\left(\mathbf{q},\omega\right)=-\frac{c}{4\pi}K_{\mu\nu}\left(\mathbf{q},\omega\right)A_{\nu}\left(\mathbf{q},\omega\right), \tag{S25}$$

where the kernel $K_{\mu\nu}\left(\mathbf{q},\omega\right)$ can be written using only the paramagnetic component [22]

$$K_{\mu\nu}\left(\mathbf{q},\omega\right)=K^{sp}_{\mu\nu}\left(\mathbf{q},\omega\right)-K^{np}_{\mu\nu}\left(\mathbf{q},0\right), \tag{S26}$$

where the first (second) term is for superconducting (normal) state. The paramagnetic kernel can be written using temperature current commutator

$$K^{sp}_{\mu\nu}\left(\mathbf{q},\omega\right)=\frac{4\pi}{\hbar c^{2}}P_{\mu\nu}\left(\mathbf{q},\omega+i\delta\right), \tag{S27}$$

where

$$P_{\mu\nu}\left(\mathbf{q},i\Omega\right)=\frac{e^{2}k_{B}T}{\hbar}\int\frac{d^{2}\mathbf{k}}{\left(2\pi\right)^{2}}\sum_{n}\mathrm{Tr}\left[\gamma_{\mu}\left(\mathbf{k},\mathbf{k}+\mathbf{q}\right)G\left(i\omega_{n}+i\Omega,\mathbf{k}+\mathbf{q}\right)\gamma_{\mu}\left(\mathbf{k}+\mathbf{q},\mathbf{k}\right)G\left(i\omega_{n},\mathbf{k}\right)\right], \tag{S28}$$

and $\gamma_{\mu}\left(\mathbf{k},\mathbf{k}+\mathbf{q}\right)$ is the velocity operator

$$\gamma_{\mu}\left(\mathbf{k},\mathbf{k}+\mathbf{q}\right)=\frac{1}{2\hbar}\left[\nabla_{\mathbf{k}+\mathbf{q}}\epsilon_{\mathbf{k}+\mathbf{q}}+\nabla_{\mathbf{k}}\epsilon_{\mathbf{k}}\right]_{\mu}=\frac{\hbar}{m}\left(k_{\mu}+\frac{q_{\mu}}{2}\right)\pm\frac{\lambda_{so}}{2\hbar}\left(\frac{k_{\mu}}{k}+\frac{k_{\mu}+q_{\mu}}{\left|\mathbf{k}+\mathbf{q}\right|}\right). \tag{S29}$$

Carrying out the Matsubara sums and after some manipulations we get

$$\begin{aligned}P_{\mu\nu}\left(\mathbf{q},i\Omega\right)=&-e^{2}\hbar\int\frac{d^{2}\mathbf{k}}{\left(2\pi\right)^{2}}\left[\frac{\hbar k_{\mu}}{m}\pm\frac{\lambda_{so}}{2\hbar}\left(\frac{k_{-\mu}}{k_{-}}+\frac{k_{+\mu}}{k_{+}}\right)\right]\left[\frac{\hbar k_{\nu}}{m}\pm\frac{\lambda_{so}}{2\hbar}\left(\frac{k_{-\nu}}{k_{-}}+\frac{k_{+\nu}}{k_{+}}\right)\right]\times\\&\left[\frac{\frac{1}{2}\left(1+\frac{\epsilon_{+}}{\xi_{+}}\right)\left(1+\frac{\epsilon_{-}}{\xi_{-}}\right)+\frac{\Delta^{2}\cos(\theta_{+}-\theta_{-})}{2\xi_{+}\xi_{-}}}{i\hbar\Omega-\left(E^{\mp,+}_{+}-E^{\mp,+}_{-}\right)}\left(f\left(E^{\mp,+}_{+}\right)-f\left(E^{\mp,+}_{-}\right)\right)+\frac{\frac{1}{2}\left(1-\frac{\epsilon_{+}}{\xi_{+}}\right)\left(1-\frac{\epsilon_{-}}{\xi_{-}}\right)+\frac{\Delta^{2}\cos(\theta_{+}-\theta_{-})}{2\xi_{+}\xi_{-}}}{i\hbar\Omega-\left(E^{\mp,-}_{+}-E^{\mp,-}_{-}\right)}\times\right.\\&\left(f\left(E^{\mp,-}_{+}\right)-f\left(E^{\mp,-}_{-}\right)\right)+\frac{\frac{1}{2}\left(1+\frac{\epsilon_{+}}{\xi_{+}}\right)\left(1-\frac{\epsilon_{-}}{\xi_{-}}\right)-\frac{\Delta^{2}\cos(\theta_{+}-\theta_{-})}{2\xi_{+}\xi_{-}}}{i\hbar\Omega-\left(E^{\mp,+}_{+}-E^{\mp,-}_{-}\right)}\left(f\left(E^{\mp,+}+_{+}\right)-f\left(E^{\mp,-}_{-}\right)\right)+\\&\left.\frac{\frac{1}{2}\left(1-\frac{\epsilon_{+}}{\xi_{+}}\right)\left(1+\frac{\epsilon_{-}}{\xi_{-}}\right)-\frac{\Delta^{2}\cos(\theta_{+}-\theta_{-})}{2\xi_{+}\xi_{-}}}{i\hbar\Omega-\left(E^{\mp,-}_{+}-E^{\mp,+}_{-}\right)}\left(f\left(E^{\mp,-}_{+}\right)-f\left(E^{\mp,+}_{-}\right)\right)\right],\end{aligned} \tag{S30}$$

where $\pm$ subscripts correspond to the momentum $\mathbf{k}_{\pm}\rightarrow\mathbf{k}\pm\frac{\mathbf{q}}{2}$ and similarly for energies, $f(x)=1/\left(e^{x/k_{B}T}+1\right)$ is the Fermi-Dirac distribution.

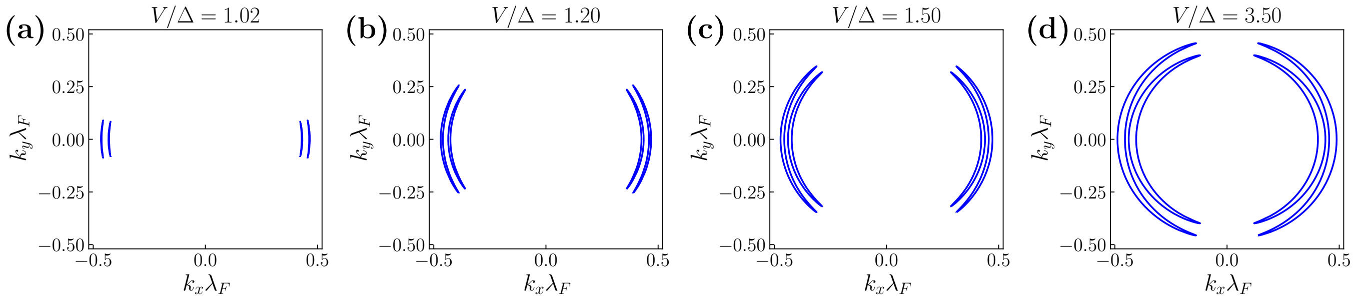


Figure S14: Bogoliubov-Fermi surfaces for different values of the Zeeman field $V$ with $\mu/\Delta=30$ obtained from the solution of Hamiltonian (S18).

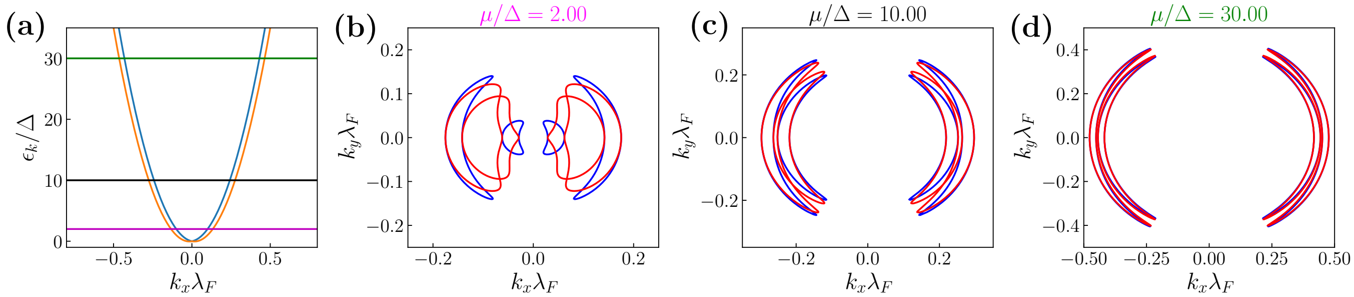


Figure S15: (a) Band structure of the Eq. (S18) without superconducting pairing and in-plane field ($V = 0$). Orange and blue correspond to two different bands and horizontal lines correspond to chemical potentials for which Bogoliubov Fermi surfaces are shown in (b-d). (b-d) Bogoliubov Fermi surfaces coming from inner band for different values of the chemical potential $\mu$. Blue are from the solution of Hamiltonian (S18) and red from (S22). Value of in-plane field is fixed to $V/\Delta = 2$ in panels (b-d).

Since superfluid density is determined by $K_{\mu\nu}(\mathbf{q} \to 0, \omega \to 0)$, for that case we get

$$K_{xx}(\mathbf{q} \to 0, \omega \to 0) = \frac{8e^2 k_F \left(\hbar k_F/m \pm \lambda_{so}/\hbar\right)}{\pi \hbar c^2} \int_0^{\pi/2} d\theta \cos^2\theta \left[ \int_{x=\Delta \mp V\cos\theta}^{\infty} dx \frac{\partial f(x)}{\partial x} \frac{x \pm V\cos\theta}{\sqrt{(x \pm V\cos\theta)^2 - \Delta^2}} + \int_{x=\Delta \pm V\cos\theta}^{\infty} dx \frac{\partial f(x)}{\partial x} \frac{x \mp V\cos\theta}{\sqrt{(x \mp V\cos\theta)^2 - \Delta^2}} \right] + \frac{2e^2 k_F \left(\hbar k_F/m \pm \lambda_{so}/\hbar\right)}{\hbar c^2}, \tag{S31}$$

where the normal component of the paramagnetic kernel was obtained by setting $\Delta = 0$. To get the expression for $K_{yy}(\mathbf{q} \to 0, \omega \to 0)$ the $\cos^2\theta$ under the integration should be converted to $\sin^2\theta$. The other components of the kernel are zero. Then superfluid density $\rho_p^{xx} \propto K_{\mu\mu}(\mathbf{q} \to 0, \omega \to 0)$ and dimensionless superfluid density reads

$$n_p^{xx} = \frac{\rho_p^{xx}}{\rho_{\mathrm{InAs}}} = 1 + \frac{4}{\pi} \int_0^{\pi/2} d\theta \cos^2\theta \left[ \int_{x=\Delta + V\cos\theta}^{\infty} dx \frac{\partial f(x)}{\partial x} \frac{x - V\cos\theta}{\sqrt{(x - V\cos\theta)^2 - \Delta^2}} + \int_{x=\Delta - V\cos\theta}^{\infty} dx \frac{\partial f(x)}{\partial x} \frac{x + V\cos\theta}{\sqrt{(x + V\cos\theta)^2 - \Delta^2}} \right], \tag{S32}$$

and similarly for $n_p^{yy}$ with the exchange of $\cos^2\theta$ to $\sin^2\theta$ under the integral. In the main text we frequently refer to $n_p = n_p^{xx}$ omitting $xx$ superscript for brevity. The superfluid density component $n_p^{yy}$ can be obtained from Eq. (S32) by replacing $\cos^2\theta$ via $\sin^2\theta$.

Let us discuss some specific cases of this expression.

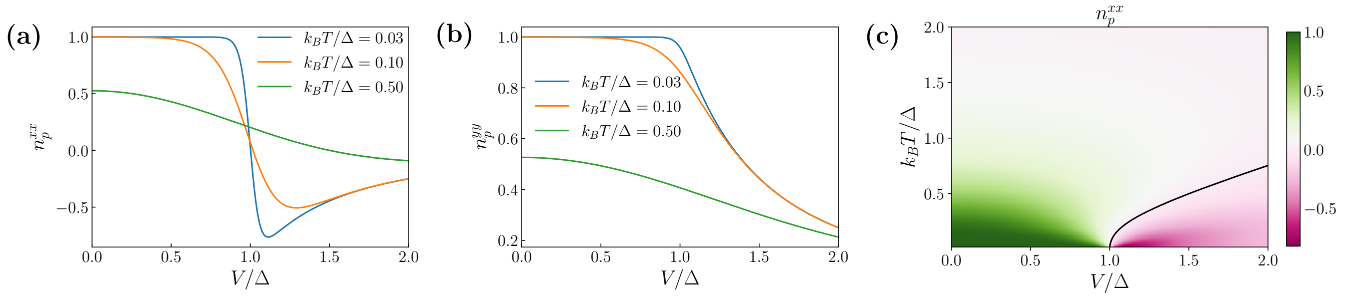


Figure S16: Normalized superfluid densities $n_p^{xx}$ (a) and $n_p^{yy}$ (b) as a function of in-plane field for different values of the temperature. (c) Color plot of superfluid density $n_p^{xx}$ direction as a function of $T$ and $V$. Black line denotes the parameter values when the superfluid density vanishes $n_p^{xx} = 0$, and separates the region of positive and negative superfluid density (on the bottom right).

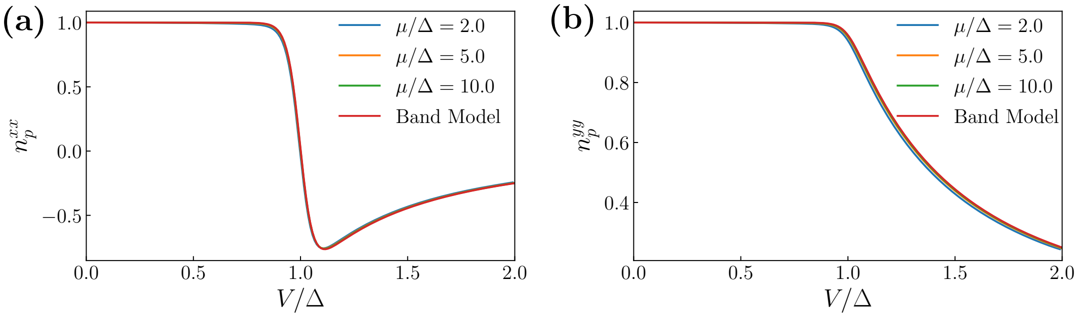


Figure S17: Superfluid density in $n_p^{xx}$ (a) and $n_p^{yy}$ (b) as a function of in-plane magnetic field calculated numerically for the full Hamiltonian (S18) for different values of $\mu$ and compared with the result of the analytic Greens function calculation, Eq. (S32). Temperature is set to $k_BT/\Delta = 0.03$ in this figure.

- When $V = 0$ the two terms in the bracket become equal and we obtain the standard BCS type expression.
- When $\Delta = 0$ and $T = 0$, the derivative of distribution function becomes a delta-function, $\partial f(x)/\partial x = -\delta(x)$, and only one of the terms in the bracket contribute, canceling the first term and resulting in $\rho_p^{xx} = 0$ as expected.
- If $V < \Delta$ and $T = 0$, the second term is zero and $\rho_p^{xx} = \rho_{\text{InAs}}$.

Fig. S16 shows the dependence of normalized superfluid densities $n_p^{xx}$ and $n_p^{yy}$ on the in-plane magnetic field parametrized by $V = g\mu_B B$ for different values of the temperature obtained from (S32). At the position when gapless Bogoliubov excitations emerge ($V > \Delta$), $n_p^{xx}$ becomes negative signaling an instability in the system that was considered previously in several different contexts [23–28]. In contrast, $n_p^{yy}$ stays always positive, which shows that electromagnetic response of the system is anisotropic. Increasing the temperature smears the Fermi-Dirac distribution function, thus shifting the position when $n_p^{xx}$ becomes negative to higher values of $V$. This can be seen more explicitly in the phase diagram on Fig. S16 (c) where $n_p^{xx} = 0$ points are shown by a black line.

Finally to see the implications of the decoupled two band model for superfluid density calculation similar to Fig. S15 for Bogoliubov Fermi surfaces, Fig. S17 compares results obtained from (S32) with the numerical evaluation of superfluid density using original Hamiltonian (S18) for different values of chemical potential $\mu$. As for the case with Bogoliubov Fermi surfaces two band model becomes precise for $\mu \gg \Delta$ and already $\mu/\Delta = 5$ is sufficient to obtain reliable results. Experimentally relevant chemical potential is approximately $\mu_{\text{exp}}/\Delta \approx 5.9 \cdot 10^3$ and the mixing between the two bands is not relevant for fitting with the experimental results.

#### 4. *Superfluid density without spin-orbit coupling*

In this section we consider electromagnetic response of 2D layer without spin-orbit coupling ($\lambda_{so} = 0$). In this case Hamiltonian (S18) separates into two sectors without further approximations. Introducing Nambu spinor $\tilde{c}_{\mathbf{k}}^\dagger = \left(c_{\mathbf{k}\uparrow}^\dagger, c_{\mathbf{k}\downarrow}^\dagger, c_{\mathbf{k}\downarrow}, -c_{\mathbf{k}\uparrow}\right)$ we can write Hamiltonian in the form

$$H(\mathbf{k}) = \epsilon(\mathbf{k})\tau^z - V\sigma^y + \Delta\tau^x, \tag{S33}$$

where in this section $\epsilon_{\mathbf{k}} = \hbar^2k^2/2m - \mu$ and $\tau$ acts in the particle-hole sector. It is clear that $H(\mathbf{k})$ commutes with $\sigma_y$ and the two sectors correspond to $\pm$ eigenvalues of $\sigma_y$. Then this Hamiltonian is identical with (S22) with $\cos\theta_{\mathbf{k}} = 1$. Therefore, we can directly write the superfluid density formula for this case as

$$n_p = 1 + \int_{x=\Delta+V}^{\infty} dx \frac{\partial f(x)}{\partial x} \frac{x - V}{\sqrt{(x-V)^2 - \Delta^2}} + \int_{x=\Delta-V}^{\infty} dx \frac{\partial f(x)}{\partial x} \frac{x + V}{\sqrt{(x+V)^2 - \Delta^2}}. \tag{S34}$$

where $\partial f(x)/\partial x = -1/(4k_BT)\,\text{sech}^2 \frac{x}{2k_BT}$ and the superfluid density is isotropic in this case.

### C. Dissipation in Al

For the varying electromagnetic fields, the absorption of the electromagnetic radiation is also a prominent phenomenon and presents further information about the system. For that we need to consider real and imaginary parts

of complex conductivity defined as

$$\sigma_{\mu\nu}(\mathbf{q},\omega) = \sigma_{1,\mu\nu}(\mathbf{q},\omega) + i\sigma_{2,\mu\nu}(\mathbf{q},\omega) = -\frac{c^2 K_{\mu\nu}(\mathbf{q},\omega)}{4\pi i\omega}. \tag{S35}$$

Using the standard results of Mattis and Bardeen in the local limit we write[29]:

$$\frac{\sigma_1(\omega)}{\sigma_n} = \frac{2}{\hbar\omega}\int_\Delta^\infty dx\,[f(x) - f(x+\hbar\omega)]\,g(x) + \frac{\Theta(\hbar\omega - 2\Delta)}{\omega}\int_{\Delta-\omega}^{-\Delta} dx\,[1 - 2f(x+\hbar\omega)]\,g(x), \tag{S36}$$

$$\frac{\sigma_2(\omega)}{\sigma_n} = \frac{1}{\hbar\omega}\int_{\max(\Delta-\hbar\omega,-\Delta)}^{\Delta} dx\,[1 - 2f(x+\hbar\omega)]\,\frac{x^2 + x\hbar\omega + \Delta^2}{\sqrt{\Delta^2 - x^2}\sqrt{(x+\hbar\omega)^2 - \Delta^2}}, \tag{S37}$$

where

$$g(x) = \frac{x^2 + x\omega + \Delta^2}{\sqrt{x^2 - \Delta^2}\sqrt{(x+\hbar\omega)^2 - \Delta^2}}. \tag{S38}$$

In the limit of $T, \hbar\omega \ll \Delta$ the Mattis-Bardeen formulas simplify to:

$$\frac{\sigma_1(\omega)}{\sigma_n} = \frac{4\Delta}{\hbar\omega} e^{-\frac{\Delta}{k_B T}} \sinh\left(\frac{\hbar\omega}{2k_B T}\right) K_0\left(\frac{\hbar\omega}{2k_B T}\right), \tag{S39}$$

$$\frac{\sigma_2(\omega)}{\sigma_n} = \frac{\pi\Delta}{\hbar\omega}\left[1 - 2e^{-\frac{\Delta}{k_B T}} e^{-\frac{\hbar\omega}{2k_B T}} I_0\left(\frac{\hbar\omega}{2k_B T}\right)\right]. \tag{S40}$$

---


[1] Anthony J Annunziata, Daniel F Santavicca, Luigi Frunzio, Gianluigi Catelani, Michael J Rooks, Aviad Frydman, and Daniel E Prober, "Tunable superconducting nanoinductors," Nanotechnology **21**, 445202 (2010).

[2] E. F. C. Driessen, P. C. J. J. Coumou, R. R. Tromp, P. J. de Visser, and T. M. Klapwijk, "Strongly disordered tin and nbtin $s$-wave superconductors probed by microwave electrodynamics," Phys. Rev. Lett. **109**, 107003 (2012).

[3] Thomas Kiendl, Felix von Oppen, and Piet W. Brouwer, "Proximity-induced gap in nanowires with a thin superconducting shell," Phys. Rev. B **100**, 035426 (2019).

[4] Yu. A. Nefyodov, A. V. Shchepetilnikov, I. V. Kukushkin, W. Dietsche, and S. Schmult, "Electron $g$-factor anisotropy in gaas/al$_{1-x}$ga$_x$as quantum wells of different symmetry," Phys. Rev. B **84**, 233302 (2011).

[5] M. D. Schroer, K. D. Petersson, M. Jung, and J. R. Petta, "Field tuning the $g$ factor in inas nanowire double quantum dots," Phys. Rev. Lett. **107**, 176811 (2011).

[6] C.L. Holloway and E.F. Kuester, "A quasi-closed form expression for the conductor loss of cpw lines, with an investigation of edge shape effects," IEEE Transactions on Microwave Theory and Techniques **43**, 2695–2701 (1995).

[7] C. H. Möller, Ch. Heyn, and D. Grundler, "Spin splitting in narrow inas quantum wells with in0.75ga0.25as barrier layers," Applied Physics Letters **83**, 2181–2183 (2003).

[8] Junsaku Nitta, Yiping Lin, Tatsushi Akazaki, and Takaaki Koga, "Gate-controlled electron g factor in an inas-inserted-channel in0.53ga0.47as/in0.52al0.48as heterostructure," Applied Physics Letters **83**, 4565–4567 (2003).

[9] Ya. V. Terent'ev, S. N. Danilov, M. V. Durnev, J. Loher, D. Schuh, D. Bougeard, S. V. Ivanov, and S. D. Ganichev, "Determination of hole g-factor in inas/ingaas/inalas quantum wells by magneto-photoluminescence studies," Journal of Applied Physics **121**, 053904 (2017).

[10] Joseph Yuan, Mehdi Hatefipour, Brenden A. Magill, William Mayer, Matthieu C. Dartiailh, Kasra Sardashti, Kaushini S. Wickramasinghe, Giti A. Khodaparast, Yasuhiro H. Matsuda, Yoshimitsu Kohama, Zhuo Yang, Sunil Thapa, Christopher J. Stanton, and Javad Shabani, "Experimental measurements of effective mass in near-surface inas quantum wells," Phys. Rev. B **101**, 205310 (2020).

[11] August E. G. Mikkelsen, Panagiotis Kotetes, Peter Krogstrup, and Karsten Flensberg, "Hybridization at superconductor-semiconductor interfaces," Phys. Rev. X **8**, 031040 (2018).

[12] Andrey E. Antipov, Arno Bargerbos, Georg W. Winkler, Bela Bauer, Enrico Rossi, and Roman M. Lutchyn, "Effects of gate-induced electric fields on semiconductor majorana nanowires," Phys. Rev. X **8**, 031041 (2018).

[13] A. I. Larkin and Y. N. Ovchinnikov, "Nonuniform state of superconductors," Zh. Eksp. Teor. Fiz. **47**, 1136–1146 (1964).

[14] Peter Fulde and Richard A. Ferrell, "Superconductivity in a strong spin-exchange field," Phys. Rev. **135**, A550–A563 (1964).

[15] M. Kjaergaard, F. Nichele, H. J. Suominen, M. P. Nowak, M. Wimmer, A. R. Akhmerov, J. A. Folk, K. Flensberg, J. Shabani, C. J. Palmstrøm, and C. M. Marcus, "Quantized conductance doubling and hard gap in a two-dimensional semiconductor–superconductor heterostructure," Nature Communications **7**, 12841 (2016).

[16] A. A. Abrikosov and L. P. Gor'kov, Sov. Phys. JETP **12**, 1243 (1961).
[17] K. Maki, *Superconductivity*, edited by R. D. Parks, Vol. II (Dekker, New York, 1969).
[18] Kazumi Maki, "The Behavior of Superconducting Thin Films in the Presence of Magnetic Fields and Currents*)," Progress of Theoretical Physics **31**, 731–741 (1964), https://academic.oup.com/ptp/article-pdf/31/5/731/5322574/31-5-731.pdf.
[19] RS Thompson and A Baratoff, "Magnetic properties of superconducting thin films in the nonlocal regime," Physical Review Letters **15**, 971 (1965).
[20] Kazumi Maki and Toshihiko Tsuneto, "Pauli Paramagnetism and Superconducting State," Progress of Theoretical Physics **31**, 945–956 (1964), https://academic.oup.com/ptp/article-pdf/31/6/945/5271369/31-6-945.pdf.
[21] Noah F. Q. Yuan and Liang Fu, "Zeeman-induced gapless superconductivity with a partial fermi surface," Phys. Rev. B **97**, 115139 (2018).
[22] Sang Boo Nam, "Theory of electromagnetic properties of superconducting and normal systems. i," Phys. Rev. **156**, 470–486 (1967).
[23] O. V. Dimitrova and M. V. Feigel'man, "Phase diagram of a surface superconductor in parallel magnetic field," Journal of Experimental and Theoretical Physics Letters **78**, 637–641 (2003).
[24] Ol'ga Dimitrova and M. V. Feigel'man, "Theory of a two-dimensional superconductor with broken inversion symmetry," Phys. Rev. B **76**, 014522 (2007).
[25] W. Vincent Liu and Frank Wilczek, "Interior gap superfluidity," Phys. Rev. Lett. **90**, 047002 (2003).
[26] Shin-Tza Wu and Sungkit Yip, "Superfluidity in the interior-gap states," Phys. Rev. A **67**, 053603 (2003).
[27] D. F. Agterberg, P. M. R. Brydon, and C. Timm, "Bogoliubov fermi surfaces in superconductors with broken time-reversal symmetry," Phys. Rev. Lett. **118**, 127001 (2017).
[28] Chandan Setty, Yifu Cao, Andreas Kreisel, Shinibali Bhattacharyya, and P. J. Hirschfeld, "Bogoliubov fermi surfaces in spin-$\frac{1}{2}$ systems: Model hamiltonians and experimental consequences," Phys. Rev. B **102**, 064504 (2020).
[29] D. C. Mattis and J. Bardeen, "Theory of the anomalous skin effect in normal and superconducting metals," Phys. Rev. **111**, 412–417 (1958).
